# Supplementary material for: Hormonal Regulation of Breast Cancer Incidence Dynamics: A Mathematical Analysis Explaining the Clemmesen's Hook
Source: arXiv:2511.19964 ancillary file (2025-11-25)
Supplement: Supplementary file 1 [file Supplements-Clemmesen.pdf]

# Supplementary Materials for Hormonal Regulation of Breast Cancer Incidence Dynamics: A Mathematical Analysis Explaining the Clemmesen's Hook

Navid Mohammad Mirzaei<sup>1\*</sup> and Wan Yang<sup>1,2\*</sup>

<sup>1\*</sup> Department of Epidemiology, Mailman School of Public Health Columbia  
University, 722 W 168th St, New York, 10032, NY, USA.

<sup>2</sup>Herbert Irving Comprehensive Cancer Center (HICCC), Columbia University Irving  
Medical Center, 630 West 168th Street, New York, 10032, NY, USA.

\*Corresponding author(s). E-mail(s): [nm3519@cumc.columbia.edu](mailto:nm3519@cumc.columbia.edu);  
[wy2202@cumc.columbia.edu](mailto:wy2202@cumc.columbia.edu);

## 1 Model Derivation

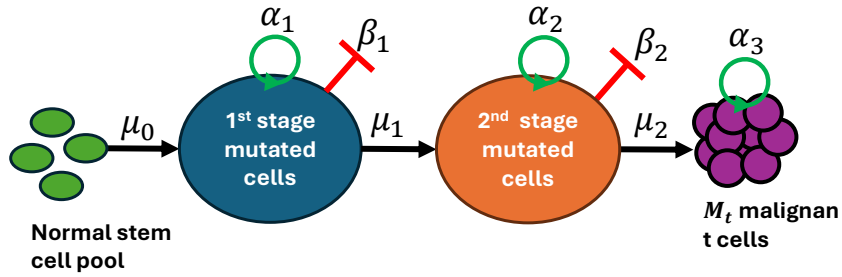

**Fig. S1** Three-stage Clonal Expansion model schematic. The incidence is equivalent to malignant cells reaching the diagnosable threshold at age  $t$ , denoted by  $M_t$ . Division rates are shown by  $\alpha_i$ , death rates by  $\beta_i$  and mutation rates by  $\mu_i$ .

The derivation here is a summarized version of the one given in our earlier study [1]. We start the derivation process by assuming that each cell undergoes only one of the transition illustrated in Figure S1 in an infinitesimally small time window  $\Delta$ . In other words, each cell

- Divides into two identical cells at a rate  $\alpha_i$  with the probability  $\alpha_i\Delta + O(\Delta^2)$ ,
- Dies at a rate  $\beta_i$  with the probability  $\beta_i\Delta + O(\Delta^2)$ ,
- Mutates at a rate  $\mu_i$  with the probability  $\mu_i\Delta + O(\Delta^2)$ ,
- Stays unchanged with the probability  $1 - (\alpha_i + \beta_i + \mu_i)\Delta + O(\Delta^2)$ .

The second order terms  $O(\Delta^2)$  are negligible, so we will omit them for the rest of the derivation. For the stem cells we assume no birth or death events given that their number stays constant ( $N_0$ ) [2] (for breast  $N_0 = 1.74 \times 10^{10}$  [3]). Also, to keep the model structurally identifiable we only consider a simple birth process for the malignant cells [1]. Let  $I_i(t)$  be the number of cells in each compartment in Figure S1 at time  $t$  for  $i = 0, 1, 2, 3$ . Defining survival as the probability of malignant cells not surpassing the diagnosable threshold  $M_t$  at age  $t$ , we have

$$P_i(t) = \Pr(I_3(t) < M_t | I_0(0) = N_0, I_1(0) = a_1, I_2(0) = a_2, I_3(0) = a_3). \quad (1)$$

Where,  $(a_1, a_2, a_3)$  is  $(0, 0, 0)$ ,  $(1, 0, 0)$ ,  $(0, 1, 0)$  and  $(0, 0, 1)$  when  $i = 0, 1, 2, 3$ , respectively. We further assume that cells in each compartment are identical and independent. The process described in figure S1 is a time homogeneous Markov process for which Chapman-Kolmogorov's law is applicable stating that for a Markov process with random variable  $X(t)$  and an event  $A$  one can write

$$\Pr(X(t+\Delta) \in A | X(0) = a) = \sum_{i=0}^{\infty} \Pr(X(t+\Delta) \in A | X(\Delta) = i) \Pr(X(\Delta) = i | X(0) = a). \quad (2)$$

Assuming infinitesimally small  $\Delta$  we have

$$\begin{aligned} P_0(t + \Delta) &= \Pr(I_3(t + \Delta) < M_{t+\Delta} | I_0(0) = N_0, I_1(0) = 0, I_2(0) = 0, I_3(0) = 0) \\ &\stackrel{\text{by (2)}}{=} \sum_{k_0, k_1, k_2, k_3} \Pr(I_3(t + \Delta) < M_{t+\Delta} | I_0(\Delta) = N_0 + k_0, I_1(\Delta) = k_1, I_2(\Delta) = k_2, I_3(\Delta) = k_3) \times \\ &\Pr(I_0(\Delta) = N_0 + k_0, I_1(\Delta) = k_1, I_2(\Delta) = k_2, I_3(\Delta) = k_3 | I_0(0) = N_0, I_1(0) = 0, I_2(0) = 0, I_3(0) = 0) \\ &= \Pr(I_3(t + \Delta) < M_{t+\Delta} | I_0(\Delta) = N_0, I_1(\Delta) = 1, I_2(\Delta) = 0, I_3(\Delta) = 0) \mu_0 N_0 \Delta + \\ &\Pr(I_3(t + \Delta) < M_{t+\Delta} | I_0(\Delta) = N_0, I_1(\Delta) = 0, I_2(\Delta) = 0, I_3(\Delta) = 0) (1 - \mu_0 N_0 \Delta) \\ &= \mu_0 N_0 P_0(t) P_1(t) \Delta + P_0(t) - \mu_0 N_0 P_0(t) \Delta \end{aligned}$$

Now we subtract  $P_0(t)$  from both sides, divide by  $\Delta$  and take the limit as  $\Delta \rightarrow 0$  to get

$$\frac{dP_0(t)}{dt} = -\mu_0 N_0 P_0(t) (1 - P_1(t)) \quad (3)$$

For  $i = 1$ , we can write

$$\begin{aligned}
P_1(t + \Delta) &= Pr(I_3(t + \Delta) < M_{t+\Delta} | I_0(0) = N_0, I_1(0) = 1, I_2(0) = 0, I_3(0) = 0) \\
&= \sum_{k_0, k_1, k_2, k_3} Pr(I_3(t + \Delta) < M_{t+\Delta} | I_0(\Delta) = N_0 + k_0, I_1(\Delta) = k_1, I_2(\Delta) = k_2, I_3(\Delta) = k_3) \times \\
&\quad Pr(I_0(\Delta) = N_0 + k_0, I_1(\Delta) = k_1, I_2(\Delta) = k_2, I_3(\Delta) = k_3 | I_0(0) = N_0, I_1(0) = 1, I_2(0) = 0, I_3(0) = 0) \\
&= Pr(I_3(t + \Delta) < M_{t+\Delta} | I_0(\Delta) = N_0, I_1(\Delta) = 1, I_2(\Delta) = 1, I_3(\Delta) = 0) \mu_1 \Delta + \\
&\quad Pr(I_3(t + \Delta) < M_{t+\Delta} | I_0(\Delta) = N_0, I_1(\Delta) = 2, I_2(\Delta) = 1, I_3(\Delta) = 0) \alpha_1 \Delta + \\
&\quad Pr(I_3(t + \Delta) < M_{t+\Delta} | I_0(\Delta) = N_0, I_1(\Delta) = 0, I_2(\Delta) = 0, I_3(\Delta) = 0) \beta_1 \Delta + \\
&\quad Pr(I_3(t + \Delta) < M_{t+\Delta} | I_0(\Delta) = N_0, I_1(\Delta) = 1, I_2(\Delta) = 0, I_3(\Delta) = 0) (1 - \mu_1 \Delta - \alpha_1 \Delta - \beta_1 \Delta) \\
&= \mu_1 P_1(t) P_2(t) \Delta + \alpha_1 P_1(t)^2 \Delta + \beta_1 \Delta + (1 - \mu_1 \Delta - \alpha_1 \Delta - \beta_1 \Delta) P_1(t).
\end{aligned}$$

Similar to (3), we can derive an ODE for  $P_1(t)$  as follows:

$$\frac{dP_1(t)}{dt} = \beta_1 - (\mu_1 + \alpha_1 + \beta_1) P_1(t) + \mu_1 P_1(t) P_2(t) + \alpha_1 P_1(t)^2. \quad (4)$$

The process for deriving the ODE for  $P_2(t)$  is identical to the above, yielding:

$$\frac{dP_2(t)}{dt} = \beta_2 - (\mu_2 + \alpha_2 + \beta_2) P_2(t) + \mu_2 P_2(t) P_3(t) + \alpha_2 P_2(t)^2. \quad (5)$$

To close the system (3)-(5) we need a closed form representation of  $P_3(t)$ . This can be obtained through the following steps:

1. Derive and solve the moment-generating PDE for a time-homogeneous birth process initiated with a single malignant cell.
2. From the obtained solution, extract the corresponding probability-generating function (PGF).
3. Compute the  $n$ -th derivative of the PGF to determine the probability of having exactly  $M_t$  malignant cells at age  $t$ .
4. Sum these probabilities from 0 to  $M_t - 1$  to obtain the probability  $P_3(t)$ .

$$P_3(t) = 1 - \left(1 - e^{-\alpha_3 t}\right)^{M_t - 1}. \quad (6)$$

A more detailed derivation of steps 1-4 can be found in our earlier study [1] or in Bailey's book [4]. These derivations are based on a general birth-death process, where the death rate of malignant cells is nonzero. The same framework can be directly applied here by setting the death rate to zero at the end of the derivation, yielding the corresponding expression for  $P_3(t)$ .

Next, we define the following instantaneous hazard:

$$h(t) = \lim_{\Delta \rightarrow 0} \frac{Pr(I_3(t) < M_t \leq I_3(t + \Delta) | I_3(t) < M_t)}{\Delta} \quad (7)$$

Using the conditional probability definition and  $Pr(I_3(t) < M_t) = 1 - Pr(I_3(t) \geq M_t)$ , we get

$$h(t) = -\frac{d}{dt} [\ln(Pr(I_3(t) < M_t))]. \quad (8)$$

Given (8) the age-specific hazard function of cancer incidence is given by the following [5].

$$\begin{aligned} h(t) &= -\frac{d}{dt} [\ln(Pr(I_3(t) < M_t | I_0(0) = N_0, I_1(0) = 0, I_2(0) = 0, I_3(0) = 0))] \\ &= -\frac{d}{dt} \ln[P_0(t)]. \end{aligned} \quad (9)$$

Finally, to be able to solve the system for the survival probabilities (3)-(5) and the hazard (9) at the same time we define the following variables:

$$\begin{aligned} x_1(t) &= P_0(t), & x_2(t) &= -\frac{d}{dt} \ln(x_1(t)), & x_3(t) &= P_1(t), \\ x_4(t) &= \dot{x}_3(t), & x_5(t) &= P_2(t), & x_6(t) &= \dot{x}_5(t), \\ f(t) &= P_3(t), \end{aligned}$$

which gives the system used in the main text.

$$\dot{x}_1 = \mu_0 N_0 x_1 (x_3 - 1), \quad (10)$$

$$\dot{x}_2 = -\mu_0 N_0 x_4, \quad (11)$$

$$\dot{x}_3 = \beta_1 - (\alpha_1 + \beta_1 + \mu_1)x_3 + \mu_1 x_3 x_5 + \alpha_1 x_3^2, \quad (12)$$

$$\dot{x}_4 = -(\alpha_1 + \beta_1 + \mu_1)x_4 + \mu_1 x_4 x_5 + \mu_1 x_3 x_6 + 2\alpha_1 x_3 x_4, \quad (13)$$

$$\dot{x}_5 = \beta_2 - (\alpha_2 + \beta_2 + \mu_2)x_5 + \mu_2 f(t) x_5 + \alpha_2 x_5^2, \quad (14)$$

$$\dot{x}_6 = -(\alpha_2 + \beta_2 + \mu_2)x_6 + \mu_2 f'(t) x_5 + \mu_2 f(t) x_6 + 2\alpha_2 x_6 x_5, \quad (15)$$

with

$$f(t) = 1 - \left(1 - e^{-\alpha_3 t}\right)^{M_t - 1}. \quad (16)$$

We have  $x_1(0) = x_3(0) = x_5(0) = 1$  given they are all survival probabilities and the rarity of germline mutation in the general population. Also assume that at age zero there is no cancer incidence  $x_2(0) = 0$ . Finally,  $x_4(0) = x_6(0) = 0$ , since they are equal to the right hand side of (12) and (14) at  $t = 0$ . This concludes our derivation for the ODE system used in the main text. Table S1 summarizes the definitions for (10)-(16).

**Table S1** Models, model variables and parameters definition.

| Variable/Parameter | Description                                                                                      |
|--------------------|--------------------------------------------------------------------------------------------------|
| $x_1$              | Survival* given $N_0$ normal cells and no other cell types at time zero.                         |
| $x_2$              | Hazard rate** of cancer incidence, i.e., $-\frac{d}{dt}[\ln x_1]$                                |
| $x_3$              | Survival given $N_0$ normal cells, one FSMC <sup>†</sup> , and no other cell types at time zero. |
| $x_4$              | Auxiliary variable defined as $\frac{d}{dt}[x_3]$                                                |
| $x_5$              | Survival given $N_0$ normal cells, one SSMC <sup>‡</sup> , and no other cell types at time zero. |
| $x_6$              | Auxiliary variable defined as $\frac{d}{dt}[x_5]$                                                |
| $N_0$              | Number of normal/stem cells;<br>$N_0 = 1.74 \times 10^{10}$ for breast [3]                       |
| $\mu_0$            | Mutation rate of normal/stem cells                                                               |
| $\mu_1$            | Mutation rate of FSMCs                                                                           |
| $\mu_2$            | Mutation rate of SSMCs                                                                           |
| $\alpha_1$         | Birth rate of FSMCs                                                                              |
| $\alpha_2$         | Birth rate of SSMCs                                                                              |
| $\alpha_3$         | Birth rate of malignant cells                                                                    |
| $\beta_1$          | Death rate of FSMCs                                                                              |
| $\beta_2$          | Death rate of SSMCs                                                                              |
| $M_t$              | Number of malignant cells at diagnosis time $t$                                                  |

\* *Survival: The probability of having less than  $M_t$  malignant cells.*

\*\* *Hazard rate: the instantaneous rate at which a specific event occurs.*

† *FSMC: First-Stage Mutated Cell*, ‡ *SSMC: Second-Stage Mutated Cell*.

## 2 Numerical Experiments

Here, we illustrate the effect of changing model parameters on the breast cancer incidence curve within and after the midlife window. We also illustrate the insensitivity of the detection dynamics within the midlife window. The results here are compared with the SEER data for the example cohort of 1935-1939.

### 2.1 Testing the Effect of Changes in Detection-related Parameters (i.e., $\alpha_3$ and $M_t$ )

Figure S2 shows the effect of scaling the detection threshold  $M_t$  and the malignant cell proliferation rate  $\alpha_3$  on the incidence in [49, 54] age window (ages when the hook is observed in the data for the cohort of 1935-1939). The baselines (dashed curves) in Figure S2 are acquired from fitting the model to the data for  $t \leq 49$  and projecting the model hazard further inside the midlife window [49, 54]. The solid blue curve is the result of the model projection when all the parameters from the baseline case are fixed and a parameter of interest is scaled within the window (i.e., increasing  $M_t$  by 10 times and reducing  $\alpha_3$  by 10-fold in the two tests, respectively). For both cases, we observe a negligible reduction in the incidence (and the L2 misfit) value, despite the unrealistic scalings we artificially imposed. These results agree with the conclusions of Theorems 5.3 and 5.4 in the main text.

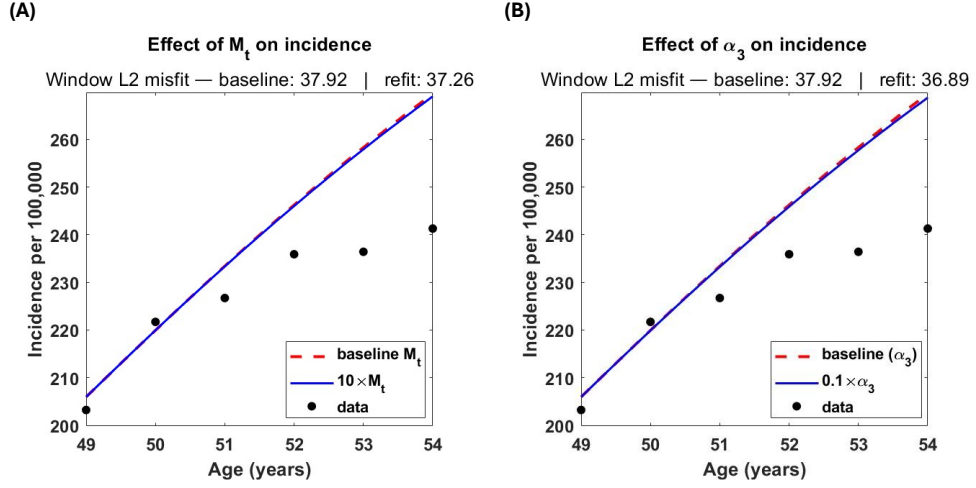

**Fig. S2** Effect of changing detection dynamics within the midlife window. (A) Incidence change from baseline by multiplying the detection threshold  $M_t$  by 10, (B) Incidence change from baseline by multiplying the malignant cells proliferation rate  $\alpha_3$  by 0.1.

## 2.2 Testing Non-detection-related Parameters for Clemmesen's Hook

Figure S3 illustrates the effect of scaling all non-detection-related parameters (i.e.,  $\mu_i$ ,  $\alpha_i$ , and  $\beta_i$ ) on the incidence within the midlife window. Again, the baseline curves are obtained by fitting the model to data for ages  $t \leq 49$  and then projecting the hazard into the midlife interval  $[49, 54]$ . The solid blue curves show the result of refitting the model to the midlife window data while varying a single parameter of interest and keeping the rest at baseline values. For each parameter re-estimation within the window, the allowable range spans from 0 to twice its baseline estimate. We can see a significant improvement for modest changes in  $\alpha_1$  and  $\beta_1$  in Figures S3 (A) and (B) with  $\alpha_1$  showing slightly better performance for less change. We also see improvement for a sizable change in  $\mu_0$  but the shape and fit improvement acquired by changing  $\alpha_1$  are still superior. The rest of the parameters do not introduce any meaningful improvements despite the drastic difference between the baseline estimates and window refit values.

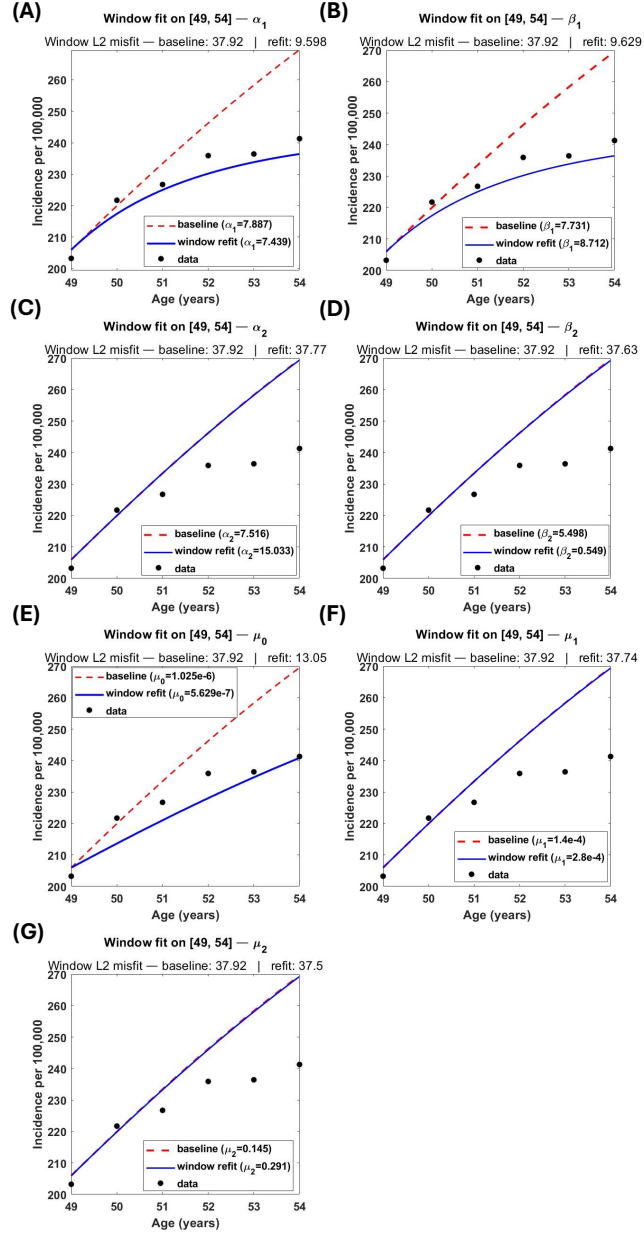

**Fig. S3** Effect of changing carcinogenic parameters within the midlife window. The panels show the change in incidence compared to the baseline estimate and the data when the model is refit on the interval [49, 54] with respect to: (A) division rate  $\alpha_1$ , (B) death rate  $\beta_1$ , (C) division rate  $\alpha_2$ , (D) death rate  $\beta_2$ , (E) mutation rate  $\mu_0$ , (F) mutation rate  $\mu_1$ , and (G) mutation rate  $\mu_2$ . See Figure S1 and Table S1 for a detailed description of the model parameters.

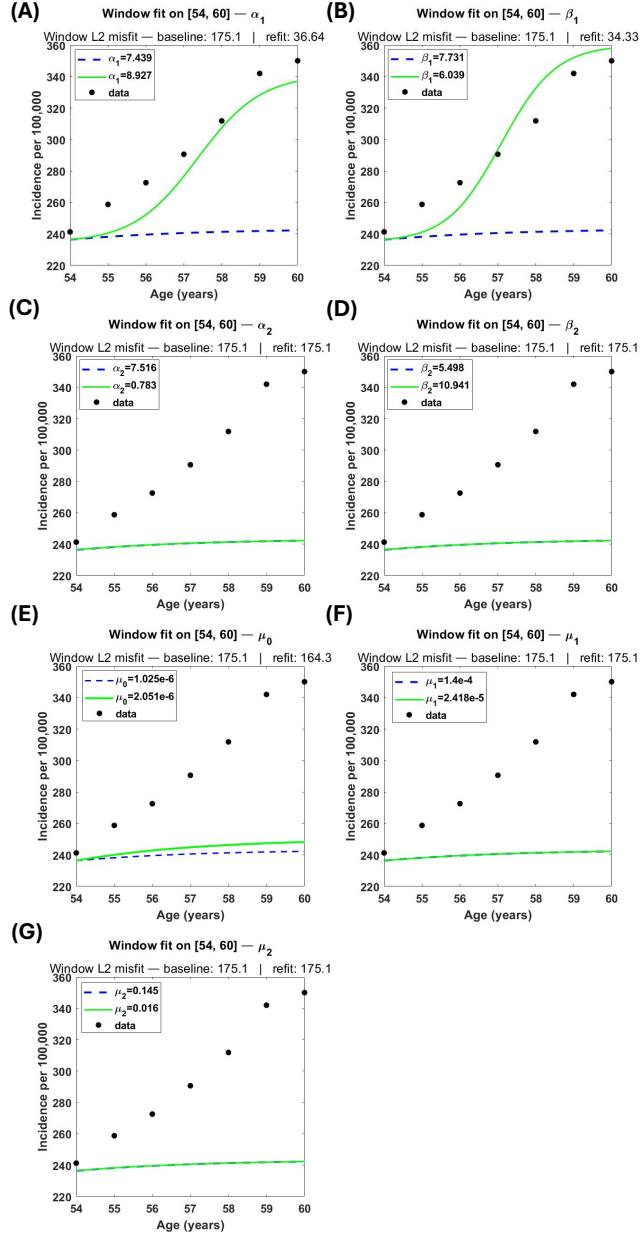

**Fig. S4** Effect of changing carcinogenic parameters after the midlife window. Shown is the change in incidence relative to the midlife window when the model is refit for  $t \geq 54$  with respect to: (A) division rate  $\alpha_1$ , (B) death rate  $\beta_1$ , (C) division rate  $\alpha_2$ , (D) death rate  $\beta_2$ , (E) mutation rate  $\mu_0$ , (F) mutation rate  $\mu_1$ , and (G) mutation rate  $\mu_2$ . See Figure S1 and Table S1 for description of the model parameters.

Figure S4 shows the effect of scaling the non-detection-related parameters on the incidence after the midlife window. For this experiment, we first fit the model to the incidence data for  $t \leq 49$  to estimate the pre-hook parameter set (as in Figure S3). All parameters are then held fixed, and a refit is performed with respect to  $\alpha_1$  alone, since it had the best performance within the midlife window. Using these parameters (i.e., pre-hook and the re-estimated  $\alpha_1$  on the midlife window), we project the hazard for  $54 \leq t \leq 60$  to generate the baseline estimates for the post-midlife window incidence (see the dashed blue lines). The solid green curves represent the result of refitting the model to the data for  $t \geq 54$  while varying a single parameter at a time and keeping all others fixed at their midlife-window values. As before, each parameter is allowed to vary within the range  $[0, 2 \times (\text{previous estimate})]$ . Consistent with earlier findings, modest adjustments to  $\alpha_1$  and  $\beta_1$  yield clear improvements (Figures S4(A)–(B)), with changing  $\beta_1$  showing slightly better performance. In contrast, changes in the remaining parameters provide no meaningful improvement, even when shifted far from their baseline values. Notably, although  $\mu_0$  could produce an incidence curve somewhat close to the midlife-window data—albeit requiring a much larger relative drop in value compared to  $\alpha_1$  and  $\beta_1$  (Figure S3(E))—it cannot rebound from the midlife dip, even when its value is doubled.

Overall, the numerical experiments in Figures S3 and S4 reinforce the theoretical conclusions of the main text: the Clemmesen’s hook can be reproduced most effectively by altering the ratio  $\alpha_1/\beta_1$ , with the strongest and most biologically plausible effects arising from first decreasing  $\alpha_1$  and then  $\beta_1$ . In contrast, although a relatively large reduction in  $\mu_0$  can generate a dip, the resulting curve does not match the data well—it lacks the characteristic curvature and fails to produce the rebound. Also, even doubling  $\mu_0$  after the dip cannot produce a rebound effect, further supporting the limited role of  $\mu_0$  in shaping the hook pattern.

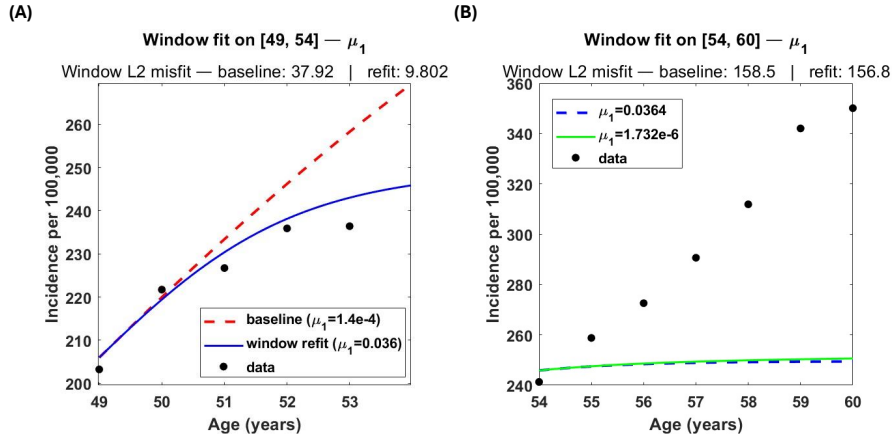

**Fig. S5** Effect of extreme changes in  $\mu_1$  value on the incidence. (A) Unrealistically extreme increase in the value of  $\mu_1$  can reproduce the dip in the midlife window. (B)  $\mu_1$  is not able to recover from the midlife dip despite an extreme decrease in value.

Finally, Figure S5 provides a numerical example demonstrating that  $\mu_1$  can generate a dip within the midlife window only under an extremely large increase—nearly a 250-fold increase (Figure S5(A)). Even more interestingly, the rebound cannot be reproduced afterward: the refit  $\mu_1$  is reduced to a value more than 20,000 times smaller but still fails to produce the post-window rebound. This further underscores that  $\mu_1$  cannot plausibly account for the Clemmesen’s hook as shown in section 6 of the main text.

## References

- [1] Mohammad Mirzaei, N., Hur, C., Terry, M.B., Dalerba, P., Yang, W.: Modeling early-onset cancer kinetics reveals changes in underlying risk and the impact of population screening. *Cancer Research* (2025)
- [2] Morrison, S.J., Shah, N.M., Anderson, D.J.: Regulatory mechanisms in stem cell biology. *Cell* **88**(3), 287–298 (1997)
- [3] Tomasetti, C., Li, L., Vogelstein, B.: Stem cell divisions, somatic mutations, cancer etiology, and cancer prevention. *Science* **355**(6331), 1330–1334 (2017)
- [4] Bailey, N.T.: *The Elements of Stochastic Processes with Applications to the Natural Sciences*. John Wiley & Sons, New York (1991)
- [5] Moolgavkar, S.H., Venzon, D.J.: Two-event models for carcinogenesis: incidence curves for childhood and adult tumors. *Mathematical biosciences* **47**(1-2), 55–77 (1979)
